# Supplementary material for: GENNI: Visualising the Geometry of Equivalences for Neural Network Identifiability
Source: arXiv:2011.07407 source file (2020-11-14)
Supplement: Supplementary file 1 [file MetaLearning.tex]

\section{Extended Applications} \label{app:extended}
In order to visualise the functionally equivalent spaces we turn our attention by investigating equivalent functions for different functions as a way to explore the applicability of our methods to transfer learning and meta-learning.

The first setting we investigate is: given a fixed number of discrete model weights sampled from $\Theta$ and a set of functions sampled from function space $\mc{F}$, we identify the subset of weight vectors that is equivalent to each of the sampled functions.  In order to investigate this, we sample five different functions, where our space of functions, $\mc{M}$, are straight lines and can be seen in figure \ref{fig:distribution}. Our model weight space $\Theta$ is 92 378 different weight vectors of one-layer feedforward neural network of 5 hidden units.

We plot a UMAP in order to visualize the underlying manifold of the equivalent weights of each function and explore the inter-relations between different functions in figure \ref{fig:multiple_functions}. It can be seen that the equivalent weights of each function lie on an underlying manifold since they follow specific patterns, i.e the equivalent weights of $y_1$ and $y_2$ lie on sub-manifolds looking like strips. Another interesting aspect is that some equivalent weight vectors of different functions lie much closer in the manifold than the rest of the equivalent weight vectors of their respective functions. This insight gave us the motivation to explore the possibility of visualizing how our framework can be used to visualize meta-learning geometrically.

In order to visualize meta-learning geometrically, we use the same 5 functions and learn a weight vector for each through gradient descent using the same one-layer neural network architecture as before. We identify other equivalent weight-vectors of each function by searching the $\epsilon$-neighbourhood of each learnt weight vector and keep only the equivalent weight-vectors for every function. Also we train the most widely used neural network meta-learning algorithm MAML \cite{MAML} on the distribution of all the straight lines. We plot a UMAP to visualize the relationship between the MAML initialization and the equivalent weight-vectors of the five functions in figure \ref{fig:umap_metal}.

From the figure it can be seen that some equivalent weight vectors from different functions lie very close to each other forming submanifolds, especially functions $y_1$ and $y_2$. Also it can be seen that the MAML initialization lies at a place where it is very close to 4 out of five equivalent weight vectors of the sampled functions. We can make a tentative assumption that MAML initialization lies at a point that is close to equivalent weight-vectors of multiple different functions.
\begin{figure}[H]
	\centering
	\begin{subfigure}{.48\textwidth}
		\centering
		\includegraphics[width=1\linewidth, height=0.2\textheight]{figures/distribution_functions.png}
		\caption{Distribution of functions}
		\label{fig:distribution}
	\end{subfigure}
		\begin{subfigure}{.48\textwidth}
		\centering
		\includegraphics[width=1\linewidth, height=0.2\textheight]{figures/5_sampled_functions.png}
		\caption{Sampled functions exploring their manifold}
	\end{subfigure}
	\begin{subfigure}{.48\textwidth}
		\centering
		\includegraphics[width=1\linewidth, height=0.2\textheight]{figures/multiple_functions_nice.png}
		\caption{UMAP of losses of the combinations of weights.}
		\label{fig:multiple_functions}
	\end{subfigure}	\begin{subfigure}{.48\textwidth}
		\centering
		\includegraphics[width=1\linewidth, height=0.2\textheight]{figures/MAML4.png}
		\caption{Equivalent functions of each of the 5 functions, along with MAML initialization bias after being trained on the whole distribution of lines}
		\label{fig:umap_metal}
	\end{subfigure}
	\caption{Exploration of equivalent functions and their relationship to meta-learning}
	\label{fig:mich_plots}
\end{figure}
